# Supplementary material for: Controllable Shadow Generation with Single-Step Diffusion Models from Synthetic Data
Source: arXiv:2412.11972 source file (2024-12-16)
Supplement: Supplementary file 2 [file appendix.tex]

\section{Appendix}
\label{sec:appendix}
